# Supplementary material for: Secrecy Energy Efficiency of MIMOME Wiretap Channels with Full-Duplex Jamming
Source: arXiv:1708.05402 source file (2019-04-30)
Supplement: Supplementary file 1 [file main_appendix.tex]

Via the application of (\ref{eq_extension_multiplelinks_aggregate_interference_covariance}), and following a similar formulation as in (\ref{error_representation_fro_norm}) we obtain 
\begin{align}
&    \sum_{k\in \mathbb{K}} \text{tr} \left({\ma{W}_i^k}^H \ma{E}_i^k\ma{W}_i^k\right) \nonumber \\ 
& =  \sum_{k \in \mathbb{K} }  \sum_{ j \in  \mathbb{I} }   \left\| \ma{c}_{ij}^k + \ma{C}_{ij}^k \text{vec}\left( \ma{\Delta}_{ij}^k \right) \right\|_{2}^2,  \label{quadratic_error_representation_final_appendix}
\end{align}
where $\ma{C}_{ij}^k$ and $\ma{c}_{ij}^k$, $j \in \{i , \bar{i} \}$ are defined similar to (\ref{calculate_c_ii})-(\ref{calculate_C_ij}). Neverthelssm for $ j \in \mathbb{I} \setminus \{i,\bar{i}\}$ the values of matrices are calculated to incorporate the impact of the additional interference terms
\begin{align}\label{calculate_c_ij_appendix}
& \ma{c}_{ij}^k \stackrel{j \in  \left\{\mathbb{I} \setminus \{i,\bar{i}\} \right\}}{:=}  \nonumber \\   &\left[ \begin{array}{c} \left\lfloor \text{vec} \left( {\ma{W}_i^k}^H {\ma{U}_i^k}^H \tilde{\ma{H}}_{ij} \left( \ma{\Theta}_{\text{tx},j}^k  \right)^{\frac{1}{2}}  \ma{\Gamma}_{N_j}^l   \ma{V}_j^m \right) \right\rfloor_{l \in \mathbb{F}_{N_j} , m \in \mathbb{K}}   \\ \left\lfloor \text{vec} \left( {\ma{W}_i^m}^H {\ma{U}_i^m}^H  \left( \ma{\Theta}_{\text{rx},i}^m  \right)^{\frac{1}{2}} \ma{\Gamma}_{M_{i}}^l \tilde{\ma{H}}_{ij}^k  \ma{V}_j^k \right) \right\rfloor_{l \in \mathbb{F}_{M_i}, m \in \mathbb{K} } \\  \text{vec}\left({\ma{W}_i^k}^H {\ma{U}_i^k}^H \tilde{\ma{H}}_{ij}^k {\ma{V}_j^k}    \right)  \end{array} \right], 
\end{align}
\begin{align}\label{calculate_C_ij_appendix}
& \ma{C}_{ij}^k \stackrel{j \in  \left\{\mathbb{I} \setminus \{i,\bar{i}\} \right\} }{:=}  \nonumber \\ &\left[ \begin{array}{c} \left\lfloor   \left(  \left( \ma{\Theta}_{\text{tx},j}^k  \right)^{\frac{1}{2}}  \ma{\Gamma}_{N_j}^{l} \ma{V}_j^m \right)^T \otimes \left( {\ma{W}_i^k}^H {\ma{U}_i^k}^H \right) \right\rfloor_{l \in \mathbb{F}_{N_j} , m\in \mathbb{K}}  \\ \left\lfloor {\ma{V}_j^k}^T \otimes \left( {\ma{W}_i^m}^H {\ma{U}_i^m}^H \left( \ma{\Theta}_{\text{rx},i}^k   \right)^{\frac{1}{2}} \ma{\Gamma}_{M_i}^l \right) \right\rfloor_{l \in \mathbb{F}_{M_i}, m \in \mathbb{K} }  \\    {\ma{V}_j^k}^T \otimes  \left( {\ma{W}_i^k}^H {\ma{U}_i^k}^H  \right)  \end{array} \right].
\end{align}
